# Supplementary material for: Molecular junctions and molecular motors: Including Coulomb repulsion in electronic friction using nonequilibrium Green's functions
Source: arXiv:1712.08061 ancillary file (2018-07-04)
Supplement: Supplementary file 1 [file SM.pdf]

# Supplementary material to: Molecular junctions and molecular motors: Including Coulomb repulsion in electronic friction using nonequilibrium Green's functions

M. Hopjan,[1,2] G. Stefanucci,[3,4,2] E. Perfetto,[5,3,2] and C. Verdozzi[1,2]

[1] *Department of Physics, Division of Mathematical Physics, Lund University, 22100 Lund, Sweden*
[2] *European Theoretical Spectroscopy Facility, ETSF*
[3] *Dipartimento di Fisica, Università di Roma Tor Vergata, Via della Ricerca Scientifica 1, 00133 Rome, Italy*
[4] *INFN, Sezione di Roma Tor Vergata, Via della Ricerca Scientifica 1, 00133 Roma, Italy*
[5] *CNR-ISM, Division of Ultrafast Processes in Materials (FLASHit), Area della Ricerca di Roma 1, Via Salaria Km 29.3, I-00016 Monterotondo Scalo, Italy*

(Dated: June 30, 2018)

## KADANOFF-BAYM EQUATIONS

The time ordered Green's function is propagated according to the Kadanoff-Baym equation [1–7] (and its adjoint)

$$\left[i\frac{d}{dt}-h_{\rm HF}(t)\right]G(t,t')=\delta(t,t')+\int_\gamma d\bar{t}\Sigma(t,\bar{t})G(\bar{t},t'),\tag{1}$$

where the integration is done along the Martin-Schwinger-Keldysh contour $\gamma$. The self-energy $\Sigma$ consists of an embedding part $\Sigma_{\rm emb.}$ describing the leads, and a correlation part $\Sigma_{\rm corr.}$ taking into account the effect of interactions. Moving from contour integration to real time integrals, the equations become

$$\left[i\frac{d}{dt}-h_{\rm HF}(t)\right]G^<(t,t')=I^<(t,t')\tag{2}$$

$$G^>(t,t')\left[i\frac{\overleftarrow{d}}{dt'}-h_{\rm HF}(t')\right]=I^>(t,t'),\tag{3}$$

with $I^{<,>}$ the collision integrals:

$$\begin{aligned}I^<(t,t')&=\int_{-\infty}^{\infty}d\bar{t}[\Sigma^<(t,\bar{t})G^A(\bar{t},t')+\Sigma^R(t,\bar{t})G^<(\bar{t},t')]\\ I^>(t,t')&=\int_{-\infty}^{\infty}d\bar{t}[G^>(t,\bar{t})\Sigma^A(\bar{t},t')+G^R(t,\bar{t})\Sigma^>(\bar{t},t')],\end{aligned}\tag{4}$$

and where the superscripts $<,>,A,R$ define lesser, greater, advanced, and retarded components of the contour ordered Green's function. The retarded Green's function satisfies the equation

$$\left[i\frac{d}{dt}-h_{\rm HF}(t)\right]G^R(t,t')=\delta(t,t')+\int d\bar{t}\Sigma^R(t,\bar{t})G^R(\bar{t},t').\tag{5}$$

We solve the Kadanoff-Baym equations with a predictor-corrector method [6, 8]. Starting from some initial value $G^<(t_{in},t_{in})$ at time $t_{in}$, the propagation to some final time $t_{max}$ requires a numerical effort which scales as $(t_{max}-t_{in})^3$ [9].

For the full Ehrenfest+KBE (EA/KBE) dynamics (where the Ehrenfest nuclear dynamics is slow and thus we must propagate the KBE for rather long times), this scaling behavior can become a severe computational limiting factor.

## GENERALIZED KADANOFF-BAYM ANSATZ

To reduce the numerical effort but keep the effects of correlations, one can consider to solve the propagation of the density matrix $\rho(t)=-iG^<(t,t)$ instead. The exact equation for $\rho(t)$ can be derived from the difference between Eq. (2) and its adjoint:

$$\frac{d\rho(t)}{dt}+i[h_{HF}(t),\rho(t)]=-(I^<(t,t)+\text{H.c.}).\tag{6}$$

This is however not a closed equation for $\rho(t)$, since Green's functions with off-diagonal time arguments appear inside the collision integral Eq. (4). To proceed, one has to reconstruct the Green's function from the density matrix. One possible way is to use the so-called Generalized Kadanoff-Baym ansatz (GKBA) [10]:

$$\begin{aligned}G^<(t,t')&=-G^R(t,t')\rho(t')+\rho(t)G^A(t,t')\\ G^>(t,t')&=+G^R(t,t')\bar{\rho}(t')-\bar{\rho}(t)G^A(t,t')\end{aligned}\tag{7}$$

where $\bar{\rho}(t)=1-\rho(t)$, and where the solution of Eq. (5) for $G^R$ needs to be further specified (see below). The GKBA reduces the numerical effort to a scaling of order $(t_{max}-t_{in})^2$, which is more favourable for the coupled Ehrenfest-GKBA (EA/GKBA) dynamics. The GKBA is then used also in the construction of the self-energy; here we work with the Second Born self-energy

$$(\Sigma^<_{\rm corr.})_{ij}(t,t')=U_iU_jG^<_{ij}(t,t')G^>_{ji}(t',t)G^<_{ij}(t,t')\tag{8}$$

and

$$\begin{aligned}(\Sigma^R_{\rm corr.})_{ij}(t,t')=U_iU_j\big(&G^R_{ij}(t,t')G^>_{ji}(t',t)G^<_{ij}(t,t')+\\ &+G^<_{ij}(t,t')G^>_{ji}(t',t)G^A_{ij}(t,t')+G^<_{ij}(t,t')G^R_{ji}(t',t)G^<_{ij}(t,t')\big).\end{aligned}\tag{9}$$

In the GKBA, the self-energy is written in terms of $\rho$ and $G^R$. The retarded self-energy is then computed via Eq. (5), which also has to be approximated, as shown next.

## STATIC-CORRELATION APPROXIMATION OF RETARDED PROPAGATOR

Here we choose to solve Eq. (5) in the static correlation limit, which was successfully tested against the full KBE solution as reported in [11]:

$$\left[i\frac{\partial}{\partial t} - h_{\rm qp}(t) - \tilde{\Sigma}^R_{\rm corr.}(t)\right] G^R(t,t') = \delta(t,t'), \tag{10}$$

where $h_{\rm qp}(t) = h_{\rm HF}(t) - i\frac{\Gamma}{2}$ and $\Gamma$ corresponds to make the Wide Band Approximation for the leads. To proceed, an adiabatic approximation is now made [11]:

$$\tilde{\Sigma}^R_{\rm corr.}(t) = \int d\bar{t}\ \tilde{\Sigma}^R_{\rm corr.}(t, t-\bar{t}) \tag{11}$$

The kernel $\tilde{\Sigma}^R_{\rm corr}(t, t-\bar{t})$ is constructed from Eq. (9) where we make use of an equilibrium propagator

$$\tilde{G}^R(t, t-t') = \int \frac{d\omega}{2\pi} \frac{e^{-i\omega(t-t')}}{\omega - h_{\rm qp}(t) - \tilde{\Sigma}^R_{\rm corr.}(t) + i\eta}. \tag{12}$$

The kernel $\tilde{\Sigma}^R_{\rm corr.}(t, t-\bar{t})$ is thus dependent implicitly on $t$ and explicitly on $t-\bar{t}$. We note that this is however only an auxiliary quantity, and not the solution of Eq. (5). As a final remark, we note that $G^R$ is fully nonadiabatic via the dependence on $h_{\rm HF}$ and the nonadiabatic $\rho$.

## GRADIENT EXPANSION RULES

*Derivative.-* The first expression which appears in the KBE and which we would like to re-express in the Wigner space [12] is the time derivative

$$\partial_{t'} = \frac{\partial T}{\partial t'}\partial_T + \frac{\partial \tau}{\partial t'}\partial_\tau = {}^1\!/\!{}_2\partial_T - \partial_\tau, \tag{13}$$

We start with the derivative acting on the two time function

$$\begin{aligned} \partial_{t'} f(t,t') &= ({}^1\!/\!{}_2\partial_T - \partial_\tau)\mathrm{f}(T,\tau) = \\ &= ({}^1\!/\!{}_2\partial_T - \partial_\tau)\int \frac{d\omega}{2\pi} e^{-i\omega\tau}\mathrm{f}(T,\omega) = \\ &= \int \frac{d\omega}{2\pi}({}^1\!/\!{}_2\partial_T + i\omega)e^{-i\omega\tau}\mathrm{f}(T,\omega) \end{aligned} \tag{14}$$

so the derivative from the KBE will be transformed as

$$-i\partial_{t'} \ \rightarrow\ (-{}^i\!/\!{}_2\partial_T + \omega) \tag{15}$$

*Integral.-* The real time integral

$$C(t,t') = \int d\bar{t} A(t,\bar{t})B(\bar{t},t') \tag{16}$$

leads in Wigner space to [13]

$$\mathrm{C}(T,\omega) = e^{-\frac{i}{2}\frac{\partial}{\partial\omega'}\frac{\partial}{\partial T} + \frac{i}{2}\frac{\partial}{\partial\omega}\frac{\partial}{\partial T'}} \mathrm{A}(T,\omega)\mathrm{B}(T',\omega')_{|\omega=\omega',T=T'}. \tag{17}$$

Doing the expansion to first order one gets

$$\begin{aligned} \mathrm{C}(T,\omega) \approx\ & \mathrm{A}(T,\omega)\mathrm{B}(T,\omega) + {}^i\!/\!{}_2[\partial_\omega \mathrm{A}(T,\omega)\partial_T \mathrm{B}(T,\omega) \\ & - \partial_T \mathrm{A}(T,\omega)\partial_\omega \mathrm{B}(T,\omega)]. \end{aligned} \tag{18}$$

*Multiplication.-* The procedure of multiplication can be reduced to the previous problem:

$$A(t,t')b(t') = \int d\bar{t} A(t,\bar{t})b(\bar{t},t')\delta(\bar{t},t'). \tag{19}$$

Using the rule in Eq. (18) for the gradient expansion derived above, the multiplication will be translated up to linear order according to

$$A(t,t')b(t') \ \rightarrow\ \mathrm{A}(T,\omega)\mathrm{b}(T) + {}^i\!/\!{}_2\partial_\omega \mathrm{A}(T,\omega)\partial_T \mathrm{b}(T). \tag{20}$$

## GRADIENT EXPANSION

In this section the self-energy $\Sigma = \Sigma_{\rm HF} + \Sigma_{\rm corr.} + \Sigma_{\rm emb.}$ contains all many-body and embedding effects, and $h$ refers to the noninteracting part.

*Retarded Green's function.-* We start with the equation of motion for the retarded Green's function in differential form

$$\begin{aligned} & -i\partial_{t'} G^R(t,t') - G^R(t,t')h(t') \\ & = \delta(t-t') + \int dt_1 G^R(t,t_1)\Sigma^R(t_1,t'), \end{aligned} \tag{21}$$

and apply the gradient expansion rules derived above so that we end up with the expression

$$\begin{aligned} & (-{}^i\!/\!{}_2\partial_T + \omega)G^R - G^R h - {}^i\!/\!{}_2\partial_\omega G^R \partial_T h \\ & \approx 1 + G^R\Sigma^R + {}^i\!/\!{}_2(\partial_\omega G^R \partial_T \Sigma^R - \partial_T G^R \partial_\omega \Sigma^R). \end{aligned} \tag{22}$$

With some algebra we get

$$\begin{aligned} & G^R(\omega - h - \Sigma^R) \approx \\ & 1 + {}^i\!/\!{}_2\partial_T G^R(1 - \partial_\omega\Sigma^R) + {}^i\!/\!{}_2\partial_\omega G^R \partial_T(h + \Sigma^R). \end{aligned} \tag{23}$$

which can be further multiplied

$$\begin{aligned} G^R \approx & [1 + {}^i\!/\!{}_2\partial_T G^R(1 - \partial_\omega\Sigma^R) + {}^i\!/\!{}_2\partial_\omega G^R \partial_T(h + \Sigma^R)] \\ & \cdot (\omega - h - \Sigma^R)^{-1}. \end{aligned} \tag{24}$$

Further we can use that $G^R \approx (\omega - h - \Sigma^R)^{-1}$ in terms already containing the time derivative

$$\begin{aligned} & G^R \approx (\omega - h - \Sigma^R)^{-1} \\ & + {}^i\!/\!{}_2[\partial_T G^R(1 - \partial_\omega\Sigma^R)G^R + \partial_\omega G^R \partial_T(h + \Sigma^R)G^R]. \end{aligned} \tag{25}$$

For the terms already containing the time derivative where $G^R \approx (\omega - h - \Sigma^R)^{-1}$ we can derive

$$\begin{aligned}\partial_\omega (G^R {G^R}^{-1}) &= \partial_\omega (G^R(\omega - h - \Sigma^R)) = \\ =&\partial_\omega G^R {G^R}^{-1} + G^R(1-\partial_\omega \Sigma^R) = 0,\end{aligned} \tag{26}$$

and thus from the last equivalence we get that the derivative with respect to $\omega$ is

$$\partial_\omega G^R = -G^R(1-\partial_\omega\Sigma^R)G^R. \tag{27}$$

Similarly we can derive the time derivative

$$\partial_T G^R = G^R \partial_T (h+\Sigma^R) G^R. \tag{28}$$

With the help of Eqs. (27, 28) can derive another useful relation:

$$\begin{aligned}&\partial_T G^R (1-\partial_\omega \Sigma^R) G^R \approx\ G^R \partial_T (h+\Sigma^R) G^R (1-\partial_\omega\Sigma^R) G^R \\ &\approx -G^R\partial_T(h+\Sigma^R)\partial_\omega G^R.\end{aligned} \tag{29}$$

The relation (29) can be used in the relation for retarded function Eq. (25) so that the final result up to linear order is in symmetric form

$$\begin{aligned}&G^R \approx (\omega - h - \Sigma^R)^{-1} \\ &+ {}^{i}\!/\!{}_{2}[\partial_\omega G^R \partial_T (h+\Sigma^R) G^R - G^R \partial_T (h+\Sigma^R)\partial_\omega G^R].\end{aligned} \tag{30}$$

*Lesser Green's function.-* We start with the equation of motion for the lesser Green's function in integral form

$$\begin{aligned}G^<(t,t') &= \int\!\!\int d\bar{t} d\bar{\bar{t}} G^R(t,\bar{t})\Sigma^<(\bar{t},\bar{\bar{t}})G^A(\bar{\bar{t}},t') \\ &= \int d\bar{t} G^R(t,\bar{t}) S^<(\bar{t},t')\end{aligned} \tag{31}$$

where $S^<(t,t') = \int d\bar{t}\Sigma^<(t,\bar{t})G^A(\bar{t},t')$ is the scattering integral. In this form we can apply the gradient expansion rule of Eq. (20) twice to get

$$\begin{aligned}G^< &\approx\ G^R S^< + {}^{i}\!/\!{}_{2}(\partial_\omega G^R \partial_T S^< - \partial_T G^R \partial_\omega S^<), \\ S^< &\approx\ \Sigma^< G^A + {}^{i}\!/\!{}_{2}(\partial_\omega \Sigma^< \partial_T G^A - \partial_T \Sigma^< \partial_\omega G^A).\end{aligned} \tag{32}$$

Plugging the expansion of $S^<$ into the expansion of $G^<$ we end up with

$$\begin{aligned}G^< &\approx G^R[\Sigma^< G^A + {}^{i}\!/\!{}_{2}(\partial_\omega\Sigma^<\partial_T G^A - \partial_T\Sigma^<\partial_\omega G^A)] + \\ &+ {}^{i}\!/\!{}_{2}(\partial_\omega G^R \partial_T[\Sigma^< G^A \ldots] - \partial_T G^R \partial_\omega[\Sigma^< G^A \ldots]).\end{aligned} \tag{33}$$

Neglecting the higher order terms in velocity and the higher order derivatives,

$$\begin{aligned}G^< \approx G^R\Sigma^< G^A &+ {}^{i}\!/\!{}_{2}[G^R\partial_\omega\Sigma^<\partial_T G^A - G^R\partial_T\Sigma^<\partial_\omega G^A \\ &+\partial_\omega G^R\partial_T\Sigma^< G^A + \partial_\omega G^R\Sigma^<\partial_T G^A - \\ &\partial_T G^R\partial_\omega\Sigma^< G^A - \partial_T G^R\Sigma^<\partial_\omega G^A].\end{aligned} \tag{34}$$

In the term $G^R\Sigma^< G^A$ we use the retarded Green's function expression of Eq. (30) to extract the terms linear in time derivatives (the same for the advanced Green's function)

$$\begin{aligned}&G^< \approx (\omega - h - \Sigma^R)^{-1}\Sigma^<(\omega - h - \Sigma^A)^{-1} \\ &+{}^{i}\!/\!{}_{2}[\partial_\omega G^R\partial_T(h+\Sigma^R)G^R - G^R\partial_T(h+\Sigma^R)\partial_\omega G^R] \\ &\quad\cdot\Sigma^<\cdot(\omega - h - \Sigma^A)^{-1} \\ &+(\omega - h - \Sigma^R)^{-1}\cdot\Sigma^<\cdot \\ &\quad{}^{i}\!/\!{}_{2}[\partial_\omega G^A\partial_T(h+\Sigma^A)G^A - G^A\partial_T(h+\Sigma^A)\partial_\omega G^A] \\ &+{}^{i}\!/\!{}_{2}[G^R\partial_\omega\Sigma^<\partial_T G^A - G^R\partial_T\Sigma^<\partial_\omega G^A + \partial_\omega G^R\partial_T\Sigma^< G^A \\ &+\partial_\omega G^R\Sigma^<\partial_T G^A - \partial_T G^R\partial_\omega\Sigma^< G^A - \partial_T G^R\Sigma^<\partial_\omega G^A].\end{aligned} \tag{35}$$

Now we can write $(\omega - h - \Sigma^{R/A})^{-1} \approx G^{R/A}$ in the terms proportional to time derivatives

$$\begin{aligned}&G^< \approx (\omega - h - \Sigma^R)^{-1}\Sigma^<(\omega - h - \Sigma^A)^{-1} \\ &+{}^{i}\!/\!{}_{2}[\partial_\omega G^R\partial_T(h+\Sigma^R)G^R\Sigma^< G^A \\ &-G^R\partial_T(h+\Sigma^R)\partial_\omega G^R\Sigma^< G^A] \\ &+{}^{i}\!/\!{}_{2}[G^R\Sigma^<\partial_\omega G^A\partial_T(h+\Sigma^A)G^A \\ &-G^R\Sigma^< G^A\partial_T(h+\Sigma^A)\partial_\omega G^A] \\ &+{}^{i}\!/\!{}_{2}[G^R\partial_\omega\Sigma^<\partial_T G^A - G^R\partial_T\Sigma^<\partial_\omega G^A + \partial_\omega G^R\partial_T\Sigma^< G^A \\ &+\partial_\omega G^R\Sigma^<\partial_T G^A - \partial_T G^R\partial_\omega\Sigma^< G^A - \partial_T G^R\Sigma^<\partial_\omega G^A].\end{aligned} \tag{36}$$

Next we use that $G^R\Sigma^< G^A \approx G^<$ in the terms proportional to time derivatives, to collect and sort all terms linear in velocity

$$\begin{aligned}&G^< \approx (\omega - h - \Sigma^R)^{-1}\Sigma^<(\omega - h - \Sigma^A)^{-1} + {}^{i}\!/\!{}_{2}[ \\ &\partial_\omega G^R\partial_T\Sigma^< G^A - G^R\partial_T\Sigma^<\partial_\omega G^A \\ &+\partial_\omega G^R\partial_T(h+\Sigma^R)G^< - G^<\partial_T(h+\Sigma^A)\partial_\omega G^A \\ &+G^R\Sigma^<\partial_\omega G^A\partial_T(h+\Sigma^A)G^A + G^R\partial_\omega\Sigma^<\partial_T G^A \\ &+\partial_\omega G^R\Sigma^<\partial_T G^A - G^R\partial_T(h+\Sigma^R)\partial_\omega G^R\Sigma^< G^A \\ &-\partial_T G^R\partial_\omega\Sigma^< G^A - \partial_T G^R\Sigma^<\partial_\omega G^A].\end{aligned} \tag{37}$$

We further work with the last three lines, where we would like to replace $\partial_T G^{R/A}$ with the relation in Eq. (29)

$$\begin{aligned}&G^< \approx (\omega - h - \Sigma^R)^{-1}\Sigma^<(\omega - h - \Sigma^A)^{-1} + {}^{i}\!/\!{}_{2}[ \\ &+\partial_\omega G^R\partial_T\Sigma^< G^A - G^R\partial_T\Sigma^<\partial_\omega G^A \\ &+\partial_\omega G^R\partial_T(h+\Sigma^R)G^< - G^<\partial_T(h+\Sigma^A)\partial_\omega G^A \\ &+(G^R\Sigma^<\partial_\omega G^A + G^R\partial_\omega\Sigma^< G^A + \partial_\omega G^R\Sigma^< G^A)\cdot \\ &\cdot\partial_T(h+\Sigma^A)G^A \\ &-G^R\partial_T(h+\Sigma^R)\cdot \\ &\cdot(\partial_\omega G^R\Sigma^< G^A - G^R\partial_\omega\Sigma^< G^A - G^R\Sigma^<\partial_\omega G^A)].\end{aligned} \tag{38}$$

Each expression in the long parenthesis in the last four lines can be rewritten with help of $\partial_\omega G^< \approx$

$\partial_\omega(G^R\Sigma^< G^A)$ so that

$$\begin{aligned}G^< \approx (\omega - h - \Sigma^R)^{-1}\Sigma^<(\omega - h - \Sigma^A)^{-1} + {}^{i}\!/\!_{2}[\\ \partial_\omega G^R \partial_T \Sigma^< G^A - G^R \partial_T \Sigma^< \partial_\omega G^A + \\ \partial_\omega G^R \partial_T (h+\Sigma^R) G^< - G^< \partial_T (h+\Sigma^A)\partial_\omega G^A + \\ +\partial_\omega G^< \partial_T (h+\Sigma^A) G^A - G^R \partial_T (h+\Sigma^R)\partial_\omega G^<].\end{aligned} \tag{39}$$

is the final expression up to linear order.

*Consistency check.*- In following we show a consistency of a relation for Green's function components

$$G^> - G^< = G^R - G^A, \tag{40}$$

with the the gradient expansions given by (30) and (39). In the consistency check we assume similar relation for the selfenergy components

$$\Sigma^> - \Sigma^< = \Sigma^R - \Sigma^A, \tag{41}$$

We start with a subtraction of the lesser component given by (39) from the greater component given by a similar equation. Then we have

$$\begin{aligned}G^> - G^< = \frac{1}{\omega - h - \Sigma^R}(\Sigma^> - \Sigma^<)\frac{1}{\omega - h - \Sigma^A} \\ + {}^{i}\!/\!_{2}[\partial_\omega G^R \partial_T (\Sigma^> - \Sigma^<) G^A \\ - G^R \partial_T (\Sigma^> - \Sigma^<)\partial_\omega G^A \\ + \partial_\omega G^R \partial_T (h+\Sigma^R)(G^> - G^<) \\ - (G^> - G^<)\partial_T (h+\Sigma^A)\partial_\omega G^A \\ + \partial_\omega (G^> - G^<) G^R \partial_T (h+\Sigma^A) G^A - \\ G^R \partial_T (h+\Sigma^R)\partial_\omega (G^> - G^<)].\end{aligned} \tag{42}$$

Now, using the relations (40) and (41) we can rewrite equaiton (42) as

$$\begin{aligned}G^> - G^< = \frac{1}{\omega - h - \Sigma^R}(\Sigma^R - \Sigma^A)\frac{1}{\omega - h - \Sigma^A} \\ + {}^{i}\!/\!_{2}[\partial_\omega G^R \partial_T (\Sigma^R - \Sigma^A) G^A \\ - G^R \partial_T (\Sigma^R - \Sigma^A)\partial_\omega G^A \\ + \partial_\omega G^R \partial_T (h+\Sigma^R)(G^R - G^A) \\ - (G^R - G^A)\partial_T (h+\Sigma^A)\partial_\omega G^A \\ + \partial_\omega (G^R - G^A) G^R \partial_T (h+\Sigma^A) G^A \\ - G^R \partial_T (h+\Sigma^R)\partial_\omega (G^R - G^A)].\end{aligned} \tag{43}$$

Expanding further we get

$$\begin{aligned}G^> - G^< = \frac{1}{\omega - h - \Sigma^R}\big[(\omega - h - \Sigma^R) \\ - (\omega - h - \Sigma^A)\big]\frac{1}{\omega - h - \Sigma^A} \\ + {}^{i}\!/\!_{2}[\partial_\omega G^R \partial_T \Sigma^R G^A - \partial_\omega G^R \partial_T \Sigma^A G^A \\ - G^R \partial_T \Sigma^R \partial_\omega G^A + G^R \partial_T \Sigma^A \partial_\omega G^A \\ + \partial_\omega G^R \partial_T (h+\Sigma^R) G^R - \partial_\omega G^R \partial_T (h+\Sigma^R) G^A \\ - G^R \partial_T (h+\Sigma^A)\partial_\omega G^A + G^A \partial_T (h+\Sigma^A)\partial_\omega G^A \\ + \partial_\omega G^R \partial_T (h+\Sigma^A) G^A - \partial_\omega G^A \partial_T (h+\Sigma^A) G^A \\ - G^R \partial_T (h+\Sigma^R)\partial_\omega G^R + G^A \partial_T (h+\Sigma^R)\partial_\omega G^R].\end{aligned}$$

Now, we group terms into parenthesis

$$\begin{aligned}G^> - G^< = \frac{1}{\omega - h - \Sigma^R} - \frac{1}{\omega - h - \Sigma^A} + {}^{i}\!/\!_{2}[ \\ \partial_\omega G^R \partial_T (h+\Sigma^R) G^R - \partial_\omega G^A \partial_T (h+\Sigma^A) G^A \\ - G^R \partial_T (h+\Sigma^R)\partial_\omega G^R + G^A \partial_T (h+\Sigma^A)\partial_\omega G^A] \\ + {}^{i}\!/\!_{2}[\partial_\omega G^R \partial_T \Sigma^R G^A - \partial_\omega G^R \partial_T \Sigma^A G^A \\ - G^R \partial_T \Sigma^R \partial_\omega G^A + G^R \partial_T \Sigma^A \partial_\omega G^A \\ + \partial_\omega G^R \partial_T (h+\Sigma^A) G^A - \partial_\omega G^R \partial_T (h+\Sigma^R) G^A \\ - G^R \partial_T (h+\Sigma^A)\partial_\omega G^A + G^A \partial_T (h+\Sigma^R)\partial_\omega G^R],\end{aligned}$$

where the terms in the second parenthesis cancel, so we finally obtain

$$\begin{aligned}G^> - G^< = \frac{1}{\omega - h - \Sigma^R} - \frac{1}{\omega - h - \Sigma^A} + {}^{i}\!/\!_{2}[ \\ \partial_\omega G^R \partial_T (h+\Sigma^R) G^R - \partial_\omega G^A \partial_T (h+\Sigma^A) G^A \\ -G^R \partial_T (h+\Sigma^R)\partial_\omega G^R + G^A \partial_T (h+\Sigma^A)\partial_\omega G^A].\end{aligned}$$

Using the relation (30) for the expansion of the retarded Green's function and a similar one for the advanced Green's function we get

$$G^> - G^< = G^R - G^A. \tag{44}$$

Thus we have shown that the gradient expansion is consistent with the relation (40).

*Short notation.*- Equations (39) and (30) can be written in short notation as

$$G^R \approx \mathrm{g}^R + \frac{\mathrm{i}}{2}\sum_\mu \dot{x}_\mu \left[\mathcal{Q}_\mu(G^R, h, G^R) + \mathcal{Q}_\mu(G^R, \Sigma^R, G^R)\right] \tag{45}$$

$$\begin{aligned}G^< \approx \mathrm{g}^R \Sigma^< \mathrm{g}^A + \frac{\mathrm{i}}{2}\dot{x}_\mu \sum_\mu \big[\mathcal{Q}_\mu(G^R, h, G^<) + \mathcal{Q}_\mu(G^<, h, G^A) + \\ \mathcal{Q}_\mu(G^R, \Sigma^R, G^<) + \mathcal{Q}_\mu(G^<, \Sigma^A, G^A) + \mathcal{Q}_\mu(G^R, \Sigma^<, G^A)\big],\end{aligned} \tag{46}$$

where

$$\mathcal{Q}_\mu(a,b,c) = [(\partial_\omega a)(\partial_{x_\mu} b)c - a(\partial_{x_\mu} b)(\partial_\omega c)], \tag{47}$$
$$\mathrm{g}^{R,A} = (\omega - h - \Sigma^{\mathrm{R,A}})^{-1}. \tag{48}$$

For later use (see e.g. the discussion below about the parameterisation of the friction coefficients), it is convenient to separate the steady-state contribution in Eq. (46):

$$G^< \approx G^<_{\mathrm{ss}} + (\mathrm{g}^R\Sigma^<\mathrm{g}^A - G^<_{\mathrm{ss}}) + \frac{\mathrm{i}}{2}\dot{x}_\mu \sum_\mu \big[\mathcal{Q}_\mu(G^R,h,G^<) + \mathcal{Q}_\mu(G^<,h,G^A) + \mathcal{Q}_\mu(G^R,\Sigma^R,G^<) + \mathcal{Q}_\mu(G^<,\Sigma^A,G^A) + \mathcal{Q}_\mu(G^R,\Sigma^<,G^A)\big]. \tag{49}$$

This permits to formally rewrite $G^<$ as

$$G^< \approx G^<_{\mathrm{ss}} + \mathrm{i}\sum_\mu \dot{x}_\mu(T)\Delta_\mu(\omega,T), \tag{50}$$

which defines the rest of the expression beyond $G^<_{\mathrm{ss}}$ as the linear term $\Delta_\mu(\omega,T)$.

In the propagator $G$, the self-energy $\Sigma = \Sigma_{\mathrm{HF}} + \Sigma_{\mathrm{corr.}} + \Sigma_{\mathrm{emb.}}$ contains all many-body and embedding effects, and $h = h(\mathbf{x}(T))$ refers to the noninteracting part. Standard conserving approximations exist to obtain $\Sigma_{\mathrm{HF}}$ and $\Sigma_{\mathrm{corr.}}$ [2]. As a side remark, we note that if, in the spirit of a steady-state density-functional theory (DFT) [14–17] , correlation effects were described in terms of exchange-correlation (XC) potential and bias ($\mathrm{V_{xc}}$,$\mathrm{b_{xc}}$), then Eq. (46) would work with $\Sigma = (\mathrm{V_H} + \mathrm{V_{xc}})[\mathbf{x}(T)] + \Sigma_{\mathrm{emb}}[\mathrm{b_{xc}}[\mathbf{x}(T)]]$ ($\mathrm{V_H}$ is the Hartree potential). Including correlations via DFT can be challenging, due the difficulty to determine the exchange-correlations correction $\Sigma_{\mathrm{emb}}[\mathrm{b_{xc}}[\mathbf{x}(T)]]$ due to the bias in the leads, and thus it seems preferable to rely on approximate self-energy schemes rather than make use of DFT.

## FRICTION PARAMETRIZATION

To proceed further we evaluate $\Delta_\mu(\omega,T)$ as defined in (49) at the steady-state Green's function, thus obtaining:

$$\dot{x}_\mu\Delta_\mu(\omega,T) \to \dot{x}_\mu\Delta_{\mu,\mathrm{ss}}(\omega) \approx -\mathrm{i}(\mathrm{g}^R_{\mathrm{ss}}\Sigma^<_{\mathrm{ss}}\mathrm{g}^A_{\mathrm{ss}} - G^<_{\mathrm{ss}}) + \frac{1}{2}\dot{x}_\mu \sum_\mu \big[\mathcal{Q}_\mu(G^R_{\mathrm{ss}},h,G^<_{\mathrm{ss}}) + \mathcal{Q}_\mu(G^<_{\mathrm{ss}},h,G^A_{\mathrm{ss}}) + \mathcal{Q}_\mu(G^R_{\mathrm{ss}},\Sigma^R_{\mathrm{ss}},G^<_{\mathrm{ss}}) + \mathcal{Q}_\mu(G^<_{\mathrm{ss}},\Sigma^A_{\mathrm{ss}},G^A_{\mathrm{ss}}) + \mathcal{Q}_\mu(G^R_{\mathrm{ss}},\Sigma^<_{\mathrm{ss}},G^A_{\mathrm{ss}})\big], \tag{51}$$

where the first term becomes zero, and we finally have

$$\Delta_{\mu,\mathrm{ss}}(\omega) \approx \frac{1}{2}\sum_\mu \big[\mathcal{Q}_\mu(G^R_{\mathrm{ss}},h,G^<_{\mathrm{ss}}) + \mathcal{Q}_\mu(G^<_{\mathrm{ss}},h,G^A_{\mathrm{ss}}) + \mathcal{Q}_\mu(G^R_{\mathrm{ss}},\Sigma^R_{\mathrm{ss}},G^<_{\mathrm{ss}}) + \mathcal{Q}_\mu(G^<_{\mathrm{ss}},\Sigma^A_{\mathrm{ss}},G^A_{\mathrm{ss}}) + \mathcal{Q}_\mu(G^R_{\mathrm{ss}},\Sigma^<_{\mathrm{ss}},G^A_{\mathrm{ss}})\big]. \tag{52}$$

The friction+Lorentz-like force is then parametrized according to:

$$F^{\mathrm{fric}}_\nu[\mathbf{x}] = 2\sum_\mu \dot{x}_\mu \int \frac{d\omega}{2\pi}\mathrm{Tr}\left[\Delta_{\mu,\mathrm{ss}}[\mathbf{x}](\omega)\partial_{x_\nu}h(\mathbf{x})\right] \equiv \sum_\mu \dot{x}_\mu\gamma_{\nu\mu}. \tag{53}$$

The friction coefficients then read

$$\gamma_{\nu\mu} = \int \frac{d\omega}{2\pi}\mathrm{Tr}\Big[\Big(\mathcal{Q}_\mu(G^R_{\mathrm{ss}}, h + \Sigma^R_{\mathrm{ss}}, G^<_{\mathrm{ss}}) + \mathcal{Q}_\mu(G^<_{\mathrm{ss}}, h + \Sigma^A_{\mathrm{ss}}, G^A_{\mathrm{ss}}) + \mathcal{Q}_\mu(G^R_{\mathrm{ss}}, \Sigma^<_{\mathrm{ss}}, G^A_{\mathrm{ss}})\Big)(\partial_{x_\nu}h)\Big]. \tag{54}$$

To highlight the effect of correlations we rewrite the expression as ($\Sigma_{\mathrm{emb.}}$ does not depend on $\mathbf{x}$ so it does not contribute in the expression)

$$\gamma_{\nu\mu} = \int \frac{d\omega}{2\pi}\mathrm{Tr}\Big[\Big(\mathcal{Q}_\mu(G^R_{\mathrm{ss}}, h_{\mathrm{HF}} + \Sigma^R_{\mathrm{ss,corr.}}, G^<_{\mathrm{ss}}) + \mathcal{Q}_\mu(G^<_{\mathrm{ss}}, h_{\mathrm{HF}} + \Sigma^A_{\mathrm{ss,corr.}}, G^A_{\mathrm{ss}}) + \mathcal{Q}_\mu(G^R_{\mathrm{ss}}, \Sigma^<_{\mathrm{ss,corr.}}, G^A_{\mathrm{ss}})\Big)(\partial_{x_\nu}h)\Big]. \tag{55}$$

This result correctly reduces to the noninteracting formula [18–20] for $h_{\mathrm{HF}} + \Sigma^{R/A}_{\mathrm{ss,corr.}} = h$ and $\Sigma^<_{\mathrm{ss,corr.}} = 0$.

## FRICTION FORMULATIONS IN LITERATURE

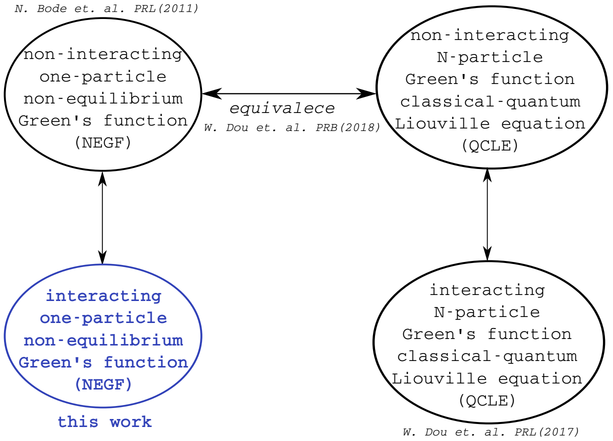


FIG. 1. Different formulations available in the literature for the non-equilibrium electronic friction. The formulation given in the present work, Eq. (55), is a generalization of the electronic friction by Bode et. al. [18]. Our formulation, in its full generality, provides an important alternative to the friction tensor of Dou et. al. [21]. The two formulations were proven to be equivalent for non-interacting systems [22].

## STEADY-STATE KBE

We solve the steady state Kadanoff-Baym equations,

$$G^R_{\rm ss} = (\omega - h - \Sigma^R_{\rm ss})^{-1}$$
$$G^<_{\rm ss} = (\omega - h - \Sigma^R_{\rm ss})^{-1}\Sigma^<_{\rm ss}(\omega - h - \Sigma^A_{\rm ss})^{-1}, \quad (56)$$

where the retarded self-energy $\Sigma^R_{\rm ss} = \Sigma^R_{\rm emb.} + \Sigma^R_{\rm ss,HF}[G] + \Sigma^R_{\rm ss,corr.}[G]$ can be divided into an embedding part, a Hartree-Fock part and a correlation part. The lesser self-energy reads $\Sigma^<_{\rm ss} = \Sigma^<_{\rm emb.} + \Sigma^<_{\rm ss,corr.}[G]$. The Hartree-Fock and correlation parts are generally dependent on the Green's function and must be solved self-consistently. For the Hubbard onsite interaction the Hartree Fock self-energy can be written as $(\Sigma^R_{\rm ss,HF})_{ij}(\omega) = \delta_{ij}U_i(n_{\rm ss})_i$ where $U_i$ is the onsite interaction and $n_{\rm ss}$ the steady-state occupation belonging to a single spin component.

*Second Born approximation (2BA)* - We use selfconsistently dressed perturbative expansion up to second order, see Fig. 2. The 2BA includes effects beyond the mean-field Hartree Fock approximation since two electrons, in addition to feel a mean-field generated by all other electrons, can also scatter directly once.

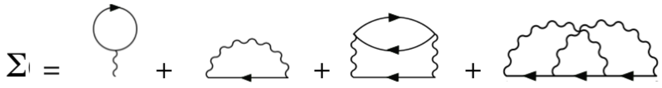

FIG. 2. The diagrams included in the 2BA. The first two diagrams are the Hartree and exchange diagrams, the third diagram is the first bubble diagram of the screened interaction series and the fourth diagram is the second-order exchange.

Evaluating the second order Feynman diagrams, the lesser part reads

$$\begin{aligned}(\Sigma^R_{\rm ss,corr.})_{ij}(\omega) = U_iU_j \int\int \frac{d\omega' d\omega''}{(2\pi)^2}\Big(&\\ (G^R_{\rm ss})_{ij}(\omega')(G^<_{\rm ss})_{ji}(\omega'')(G^<_{\rm ss})_{ij}(\omega-\omega'+\omega'')+&\\ +\,(G^R_{\rm ss})_{ij}(\omega')(G^<_{\rm ss})_{ji}(\omega'')(G^R_{\rm ss})_{ij}(\omega-\omega'+\omega'')-&\\ -\,(G^R_{\rm ss})_{ij}(\omega')(G^<_{\rm ss})_{ji}(\omega'')(G^R_{\rm ss})^*_{ji}(\omega-\omega'+\omega'')+&\\ +\,(G^<_{\rm ss})_{ij}(\omega')(G^R_{\rm ss})^*_{ij}(\omega'')(G^<_{\rm ss})_{ij}(\omega-\omega'+\omega'')+&\\ +\,(G^<_{\rm ss})_{ij}(\omega')(G^<_{\rm ss})_{ji}(\omega'')(G^R_{\rm ss})_{ij}(\omega-\omega'+\omega'')\Big).&\end{aligned} \quad (57)$$

For the retarded part, we have instead

$$\begin{aligned}(\Sigma^<_{\rm ss,corr.})_{ij}(\omega) = U_iU_j \int\int \frac{d\omega' d\omega''}{(2\pi)^2}\Big(&\\ (G^<_{\rm ss})_{ij}(\omega')(G^<_{\rm ss})_{ji}(\omega'')(G^<_{\rm ss})_{ij}(\omega-\omega'+\omega'')+&\\ +\,(G^<_{\rm ss})_{ij}(\omega')(G^R_{\rm ss})_{ji}(\omega'')(G^<_{\rm ss})_{ij}(\omega-\omega'+\omega'')-&\\ -\,(G^<_{\rm ss})_{ij}(\omega')(G^R_{\rm ss})^*_{ij}(\omega'')(G^<_{\rm ss})_{ij}(\omega-\omega'+\omega'')\Big).&\end{aligned} \quad (58)$$

*T matrix approximation (TMA)* - The TMA includes the same effects as the 2BA plus a higher order multiple electron-electron scattering. In this approximation we construct two-particle propagators [8]

$$\begin{aligned}(\mathcal{G}^<_{\rm ss})_{ij}(\omega) &= \int \frac{d\omega'}{2\pi}\Big((G^<_{\rm ss})_{ij}(\omega')(G^<_{\rm ss})_{ij}(\omega-\omega')\Big),\\ (\mathcal{G}^R_{\rm ss})_{ij}(\omega) &= \int \frac{d\omega'}{2\pi}\Big((G^R_{\rm ss})_{ij}(\omega')(G^<_{\rm ss})_{ij}(\omega-\omega')+\\ &\quad +(G^R_{\rm ss})_{ij}(\omega')(G^R_{\rm ss})_{ij}(\omega-\omega')+\\ &\quad +(G^<_{\rm ss})_{ij}(\omega')(G^R_{\rm ss})_{ij}(\omega-\omega')-\\ &\quad -(G^R_{\rm ss})_{ij}(\omega')(G^R_{\rm ss})^*_{ji}(\omega-\omega')\Big),\end{aligned} \quad (59)$$

and we find the T matrix from Dyson-like equations:

$$\begin{aligned}\big(U*\mathcal{G}^R_{\rm ss}\big)_{ij}(\omega) &= \sum_l U_{il}(\mathcal{G}^R_{\rm ss})_{lj}(\omega)\\ \big(T^R_{\rm ss}\big)_{ij}(\omega) &= -i\sum_l \big(\big(\delta - iU*\mathcal{G}^R_{\rm ss}\big)^{-1}\big)_{il}(\omega)\;U_{lj}\\ \big(T^<_{\rm ss}\big)_{ij}(\omega) &= \sum_{kl}\big(T^R_{\rm ss}\big)_{ik}(\omega)\big(\mathcal{G}^<_{\rm ss}\big)_{kl}(\omega)\big(T^R_{\rm ss}\big)^*_{jl}(\omega).\end{aligned} \quad (60)$$

The lesser self-energy is obtained from the T-matrix via

$$\begin{aligned}(\Sigma^<_{\rm ss,corr})_{ij}(\omega) = \int\frac{d\omega'}{2\pi}\Big(&(G^<_{\rm ss})_{ji}(\omega')(T^<_{\rm ss})_{ij}(\omega+\omega')\\ &+(G^R_{\rm ss})_{ji}(\omega')(T^<_{\rm ss})_{ij}(\omega+\omega')\\ &-(G^R_{\rm ss})^*_{ij}(\omega')(T^<_{\rm ss})_{ij}(\omega+\omega')\Big).\end{aligned} \quad (61)$$

For the retarded self-energy we have instead

$$\begin{aligned}(\Sigma^R_{\rm ss,HF+corr.})_{ij}(\omega) = \int\frac{d\omega'}{2\pi}\Big(&(G^<_{\rm ss})_{ji}(\omega')(T^R_{\rm ss})_{ij}(\omega+\omega')\\ &+(G^R_{\rm ss})^*_{ij}(\omega')(T^<_{\rm ss})_{ij}(\omega+\omega')\Big).\end{aligned} \quad (62)$$

We wish to stress that the Hartree Fock contribution is already included in these expressions.

## FRICTION - EFFECT OF CORRELATIONS

In Fig. 3 we show the nonequilibrium friction coefficient $\gamma_{(1)}$ for three different levels of treatment of the electronic correlations. Looking at the friction coefficient and the region of positive damping, we observe that the mean-field Hartree-Fock approximation predicts a trend opposite to those obtained from approximations accounting for correlations effects, i.e. 2BA and TMA. We thus conclude that the TMA results provide additional evidence about the importance of taking into account correlation effects.

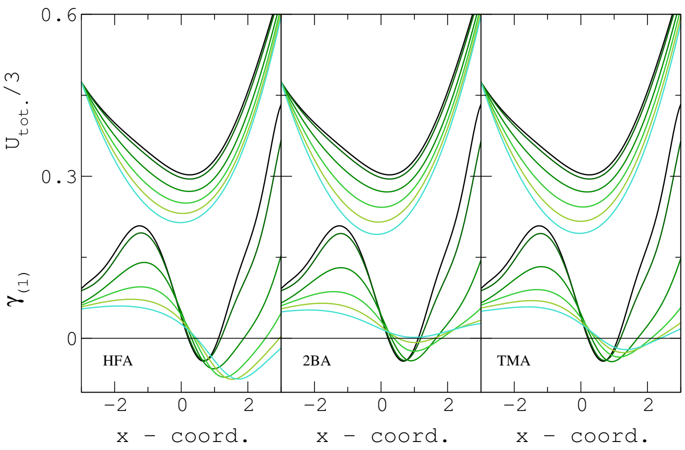


FIG. 3. The nonequilibrium potential $U_{tot.}$ and the friction $\gamma^{\mu\nu}_{(1)}$ for HFA, 2BA and TMA as a function of the interaction strength $U$. The parameters of the dimensionless Hamiltonian are (L/R=left/right): $g = \frac{\sqrt{10}}{2}$, $J_c = -3.5$, $v_c^{eq.} = 0.0$, $v_c^{noneq.} = 1.0$, $U = (0.0 - 10.0)$, $J_{L/R} = -50.0$, $J^{11_L}_{tun.} = J^{21_R}_{tun.} = -8.66$, $V^{eq.}_{L/R} = 0.0$, $V^{noneq.}_{L/R} = \pm 5.0$.

## ESTIMATES OF THE SIZES OF THE EFFECTS

Using the continuity equation the maximum current $I_{\max}$ is of the same order of magnitude of the maximum value of the time-derivative of the density. The latter can be estimated from the ratio between the amplitude $\Delta n$ of the density oscillations and half the period of these oscillations, i.e., $T/2 = \pi/\Omega$. For a normal mode with period $T$ in the physical range $5 \div 50$ fs (hence $\Omega$ in the range $20 \div 200$ THz) we find

$$I_{\max} = \frac{1.6 \times 10^{-19}\Delta n}{2.5 \times (10^{14} \div 10^{15})} \frac{\mathrm{C}}{\mathrm{s}} \approx 6\Delta n \times (10^{-5} \div 10^{-6}) \text{ A} \quad (63)$$

From Fig. 3 of the paper we see that $\Delta n$ is about $10^{-1}$ or lower. Therefore the maximum current is in the micro-Ampere range, which is the typical order of magnitude in molecular transport. The nuclear displacement $x$ is measured in units of the characteristic length $l_0 = \sqrt{\hbar/(M\Omega)}$ which depends on the mass of the dimer. As an example we can consider the ethylen molecule and take the two carbon atoms as the two sites of the dimer. Then $M = 24 \times M_{\text{proton}} = 24 \times 1.67 \times 10^{-27}$ Kg. Inserting this value in the equation for $l_0$ and taking into account that $\Omega^{-1} = T/2\pi = (5 \div 50) \times 10^{-15}$ s$/2\pi$ we find

$$l_0 \simeq \sqrt{\frac{10^{-34}\mathrm{m}^2\mathrm{Kg/s}}{24 \times 1.67 \times 10^{-27}\ \mathrm{Kg}} \frac{(5 \div 50) \times 10^{-15}\mathrm{s}}{2\pi}} \approx (10^{-1} \div 10^{-2})\text{Å} \quad (64)$$

which is in the range of physical displacements.

The physical picture is therefore that a bias difference $V_L - V_R \sim 10\hbar\Omega$ (we recall that in our simulations $V_L = -V_R = 5\hbar\Omega$, which corresponds to a few hundred of meV for $\Omega$ in the range $20 \div 200$ THz) activates a sloshing motion of the center of mass of the dimer (see Fig. 1 of the paper) which for negative $\gamma$ is ever lasting. Our results show that this electromechanical energy conversion is hampered by the Coulomb interaction.


[1] L.P. Kadanoff and G. Baym, *Quantum Statistical Mechanics* (Benjamin, New York, 1962).
[2] G. Baym and L. P. Kadanoff, Phys. Rev. **124**, 287 (1961).
[3] L.V. Keldysh, Sov. Phys. JETP **20**, 1018 (1965).
[4] G. Stefanucci and R. van Leeuwen, *Nonequilibrium Many-Body Theory of Quantum Systems: A Modern Introduction* (Cambridge University Press, Cambridge, 2013).
[5] K. Balzer and M. Bonitz, *Nonequilibrium Green's Functions Approach to Inhomogeneous Systems*, Lecture Notes in Physics Vol. 867 (Springer, Berlin, Heidelberg, 2013).
[6] M. Hopjan and C. Verdozzi, *First Principles Approaches to Spectroscopic Properties of Complex Materials* (Springer, Berlin, Heidelberg, 2014); pp.347-384.
[7] N Schlünzen, J.P. Joost, M. Bonitz, Phys. Rev. B **96**, 117101 (2017).
[8] M. Puig von Friesen, C. Verdozzi, and C.-O. Almbladh, Phys. Rev. Lett. **103**, 176404 (2009); Phys. Rev. B **82**, 155108 (2010).
[9] S. Hermanns, K. Balzer, and M. Bonitz, Phys. Scr. **T151**, 014036 (2012).
[10] P. Lipavsky, V. Spicka, and B. Velicky, Phys. Rev. B **34**, 6933 (1986).
[11] S. Latini, E. Perfetto, A.-M. Uimonen, R. van Leeuwen, G. Stefanucci, Phys. Rev. B **89**, 075306 (2014).
[12] E. Wigner, Phys. Rev. **40**, 749 (1932).
[13] J. Moyal, Proc. Cambridge Philos. Soc. **45**, 99 (1949).
[14] G. Stefanucci and S. Kurth, Nano Lett. **15**, 8020-8025 (2015).
[15] D. Karlsson and C. Verdozzi, J. Phys. conf. Ser. **696**, 012018 (2016).
[16] S. Kurth and G. Stefanucci, J. Phys: Cond. Matter, **29** (2017).
[17] D. Karlsson, M. Hopjan, and C. Verdozzi, Phys. Rev. B **97**, 125151 (2018).
[18] N. Bode, S. V. Kusminskiy, R. Egger and F. von Oppen, Phys. Rev. Lett. **107**, 036804 (2011).
[19] N. Bode, S. V. Kusminskiy, R. Egger and F. von Oppen, Beilstein J Nanotechnol. **3**, 144-162 (2012).
[20] A. Kartsev, C. Verdozzi, G. Stefanucci, EPJ B **87**, 14 (2014).
[21] W. Dou, G. Miao and J.E. Subotnik, Phys. Rev. Lett. **119**, 046001 (2017).
[22] W.Dou and J.E. Subotnik, Phys. Rev. B **97**, 064303 (2018).
